# Supplementary material for: Counterfactual-based Root Cause Analysis for Dynamical Systems
Source: arXiv:2406.08106 source file (2024-06-12)
Supplement: Supplementary file 1 [file apdx.tex]

% This is samplepaper.tex, a sample chapter demonstrating the
% LLNCS macro package for Springer Computer Science proceedings;
% Version 2.21 of 2022/01/12
%
\documentclass[runningheads]{llncs}
\usepackage[T1]{fontenc}
% T1 fonts will be used to generate the final print and online PDFs,
% so please use T1 fonts in your manuscript whenever possible.
% Other font encondings may result in incorrect characters.
%
% Used for displaying a sample figure. If possible, figure files should
% be included in EPS format.
%
% If you use the hyperref package, please uncomment the following two lines
% to display URLs in blue roman font according to Springer's eBook style:

%

%\usepackage{amsmath}
\usepackage{graphicx}
\usepackage{subfig}
\usepackage{amsfonts}
\usepackage{hyperref}
\usepackage{color}

\urlstyle{rm}
\usepackage{dsfont}
\usepackage{tabularx}
\usepackage{booktabs}
\usepackage{mathtools}
\usepackage{todonotes}
\usepackage{wrapfig}
\usepackage{xargs} 
\usepackage{multirow}
\newcommandx{\unsure}[2][1=]{\todo[linecolor=red,backgroundcolor=red!25,bordercolor=red,#1]{#2}}

\newcommandx{\tbd}[2][1=]{\todo[linecolor=red,backgroundcolor=red!25,bordercolor=red,inline,#1]{TBD: #2}}

\newcommandx{\resp}[2][1=]{\todo[linecolor=red,backgroundcolor=red!25,bordercolor=red,#1]{Responsible: #2}}

\newcommandx{\sebastian}[2][1=]{\todo[linecolor=green,backgroundcolor=green!25,bordercolor=green,inline,#1]{Sebastian: #2}}

\newcommandx{\juliane}[2][1=]{\todo[linecolor=green,backgroundcolor=green!25,bordercolor=green,#1]{Juliane: #2}}

\newcommandx{\mf}[2][1=]{\todo[linecolor=red,backgroundcolor=green!25,bordercolor=red,inline,#1]{MF: #2}}

\newcommandx{\karim}[2][1=]{\todo[linecolor=green,backgroundcolor=green!25,bordercolor=green,#1]{Karim: #2}}

\begin{document}
\institute{}
\author{Author information scrubbed for double-blind reviewing}
\title{Counterfactual-based Root Cause Analysis for Dynamical Systems - Appendix}
\maketitle

\section{Hyperparameter setup}
We report the hyperparameters of our Residual neural network in Table~(\ref{tb:hyperpara}). It consists of three layers with hyperbolic tangent activation functions and 128 neurons as latent layer. Note that we chose $\Delta_{t} = 1.0$ for all experiments.

\begin{table*}[ht]
\begin{center}
 \caption{Hyperparameter setup of \textit{NLin} for the performed experiments.} 
 %\resizebox{1\textwidth}{!}{
\begin{tabular}{lc|c|c|c|c|l}\toprule
& {Lin. system} & {FHN oscillator} & {EasyRCA benchmarking} & {River} \\\midrule
%\midrule(lr){2-2}\cmidrule(lr){3-3}\cmidrule(lr){4-4}\cmidrule(lr){5-5} \\
\textit{splits}           & 4 & 4 & 6 & 4 \\
\textit{$T_{train}$}     & 1000 & 1000 & -\protect\footnotemark & ~300.000 \\
\textit{$T_{factum}$}    & 20 & 50 & - & 90 \\
\textit{lr}               & 0.01 & 0.01 & 0.1 & 0.01\\
\textit{epochs}          & 50 & 100 & 200 & 50 \\
\textit{dim}          & 2 & 2 & 1 & 1 \\
\bottomrule
\end{tabular}
\label{tb:hyperpara}%}
\end{center}
\end{table*}
\footnotetext{In the EasyRCA benchmark the normal data and the factum have for each experiment the same length, see Table 2 in the main paper for corresponding $T$.}

\section{Linear synthetic system}
In the following we show the coefficient matrices for the data generation of the linear synthetic system. The matrix of the root node $w$ was chosen such that the eigenvalues are smaller than 1,  which guarantees a stable system. 

\begin{equation*}
    A^{ww}=
\begin{bmatrix}
0.949 & 0.313\\
-0.313 & 0.949
\end{bmatrix},
A^{xx}=
\begin{bmatrix}
0.2 & -0.1 \\
-0.1 & 0.2 
\end{bmatrix},
A^{yy}=
\begin{bmatrix}
0.2 & 0.1 \\
0.1 & 0.2 
\end{bmatrix},
A^{zz}=
\begin{bmatrix}
0.2 & 0.1 \\
0.1 & 0.2 
\end{bmatrix}
\end{equation*}

\begin{equation*}
B^{wx}=
\begin{bmatrix}
0.5 & 0.2 \\
0.2 & -0.5 
\end{bmatrix},
B^{xy}=
\begin{bmatrix}
-0.9 & 0.7 \\
0.7 & -0.9 
\end{bmatrix},
B^{xz}=
\begin{bmatrix}
0.4 & 0.9 \\
0.9 & 0.4 
\end{bmatrix},
B^{yz}=
\begin{bmatrix}
0.6 & 0.4 \\
0.4 & 0.6 
\end{bmatrix}
\end{equation*}
\begin{equation}
C^{w},C^{x},C^{y},C^{z}=
\begin{bmatrix}
0.01 & 0.01 \\
0.01 & 0.01 
\end{bmatrix}
\end{equation}

\section{FHN oscillator}
We performed the same kind of injection experiment as for the linear system. In Fig. \ref{fig:injection-boxplot-FHN}, we show varying root cause injections (varying constant added to the structural equation) over 20 randomly sampled facta with $T=50$. On the left, for \textit{NLin} it can be seen that the model intervening on the structure and the noise achieves a significantly higher identification score for larger added constants. This could be due to a large root cause, in this setting leading to a factum with high distance to the normal data, which may lead to a divergence over time of the normal behaviour system $\mathcal{M}$. On the right, we illustrated \textit{Lin} and as expected, it is inadequate for addressing the complexities of the nonlinear problem.
\subsection{Injection experiment}
\begin{figure}
    \centering
    {\includegraphics[width=0.49\textwidth]{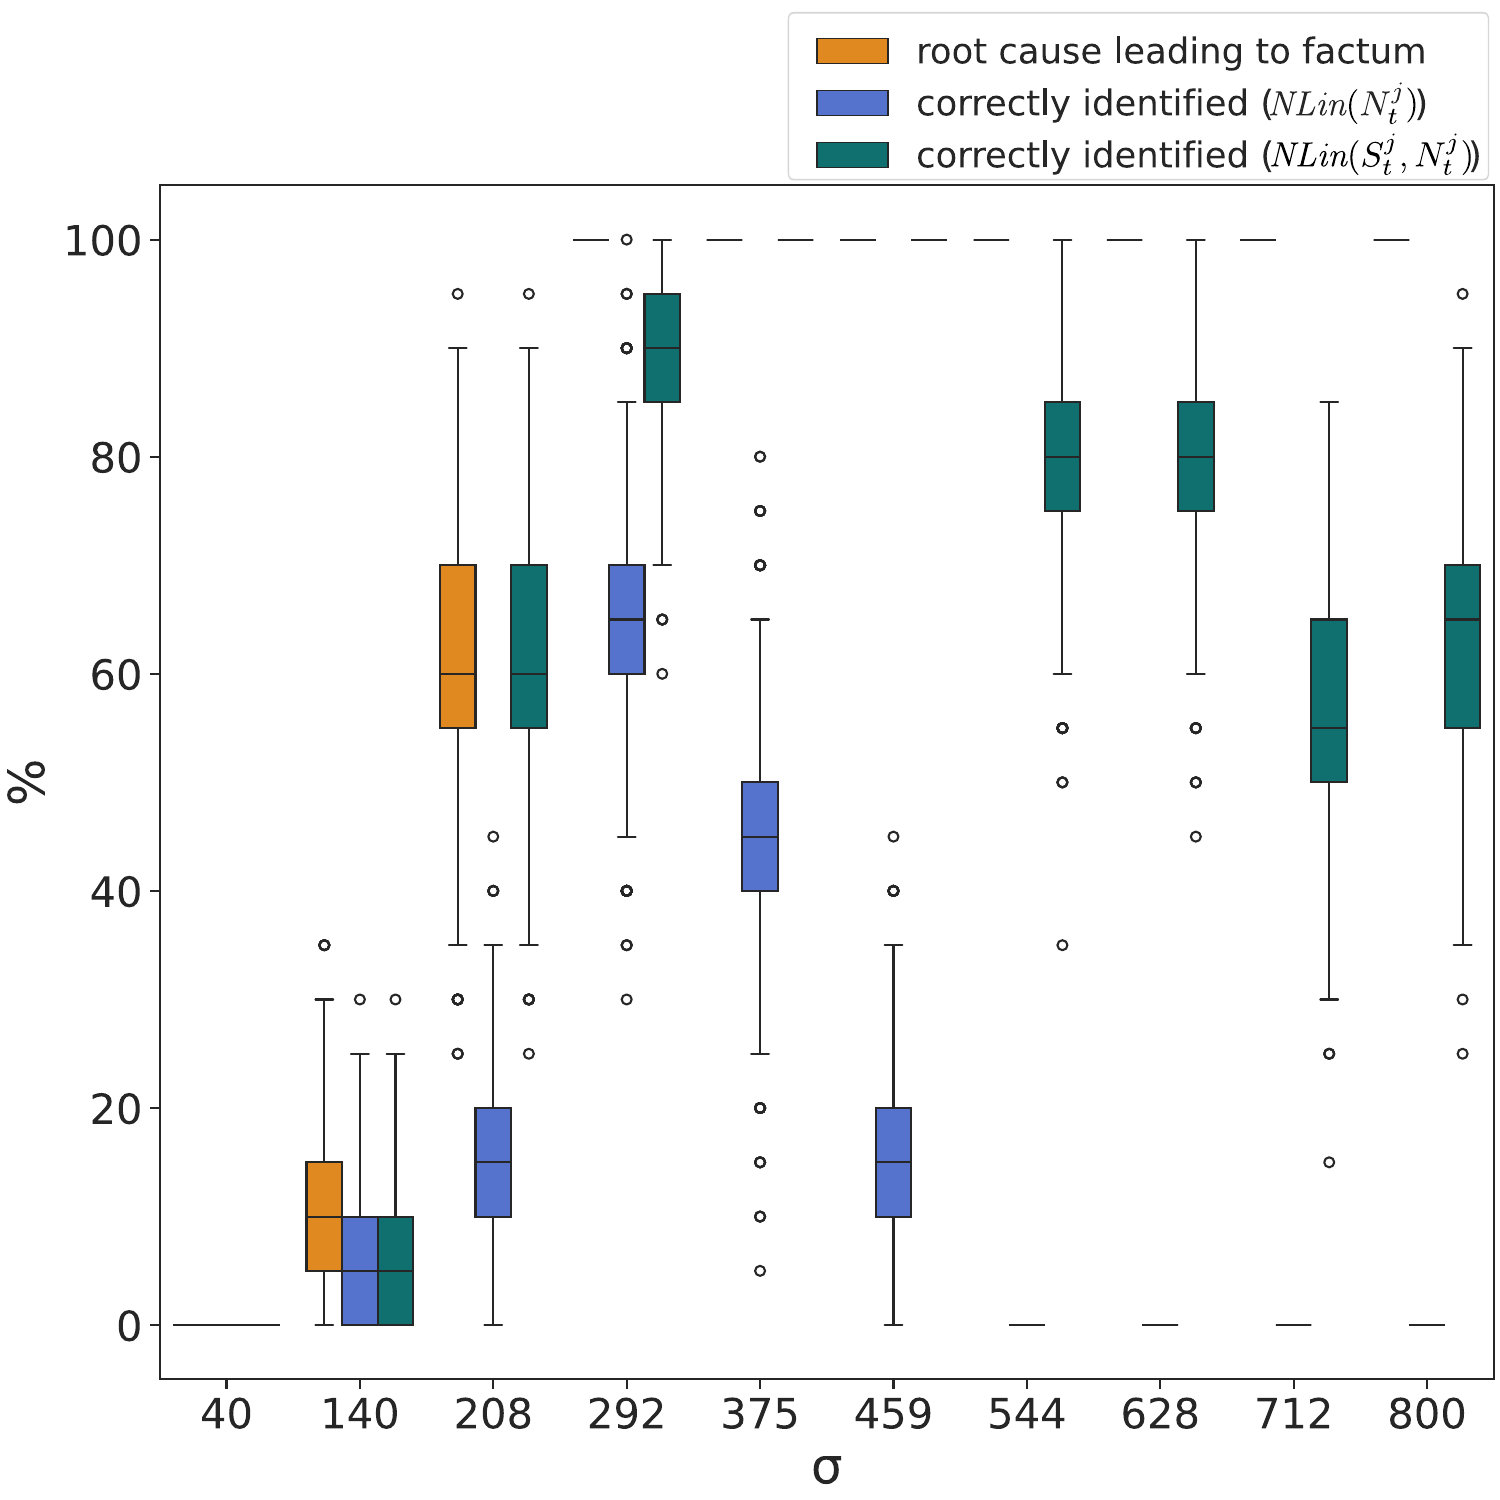}\label{fig:nl_model_oscillator_boxplot}}
    {\includegraphics[width=0.49\textwidth]{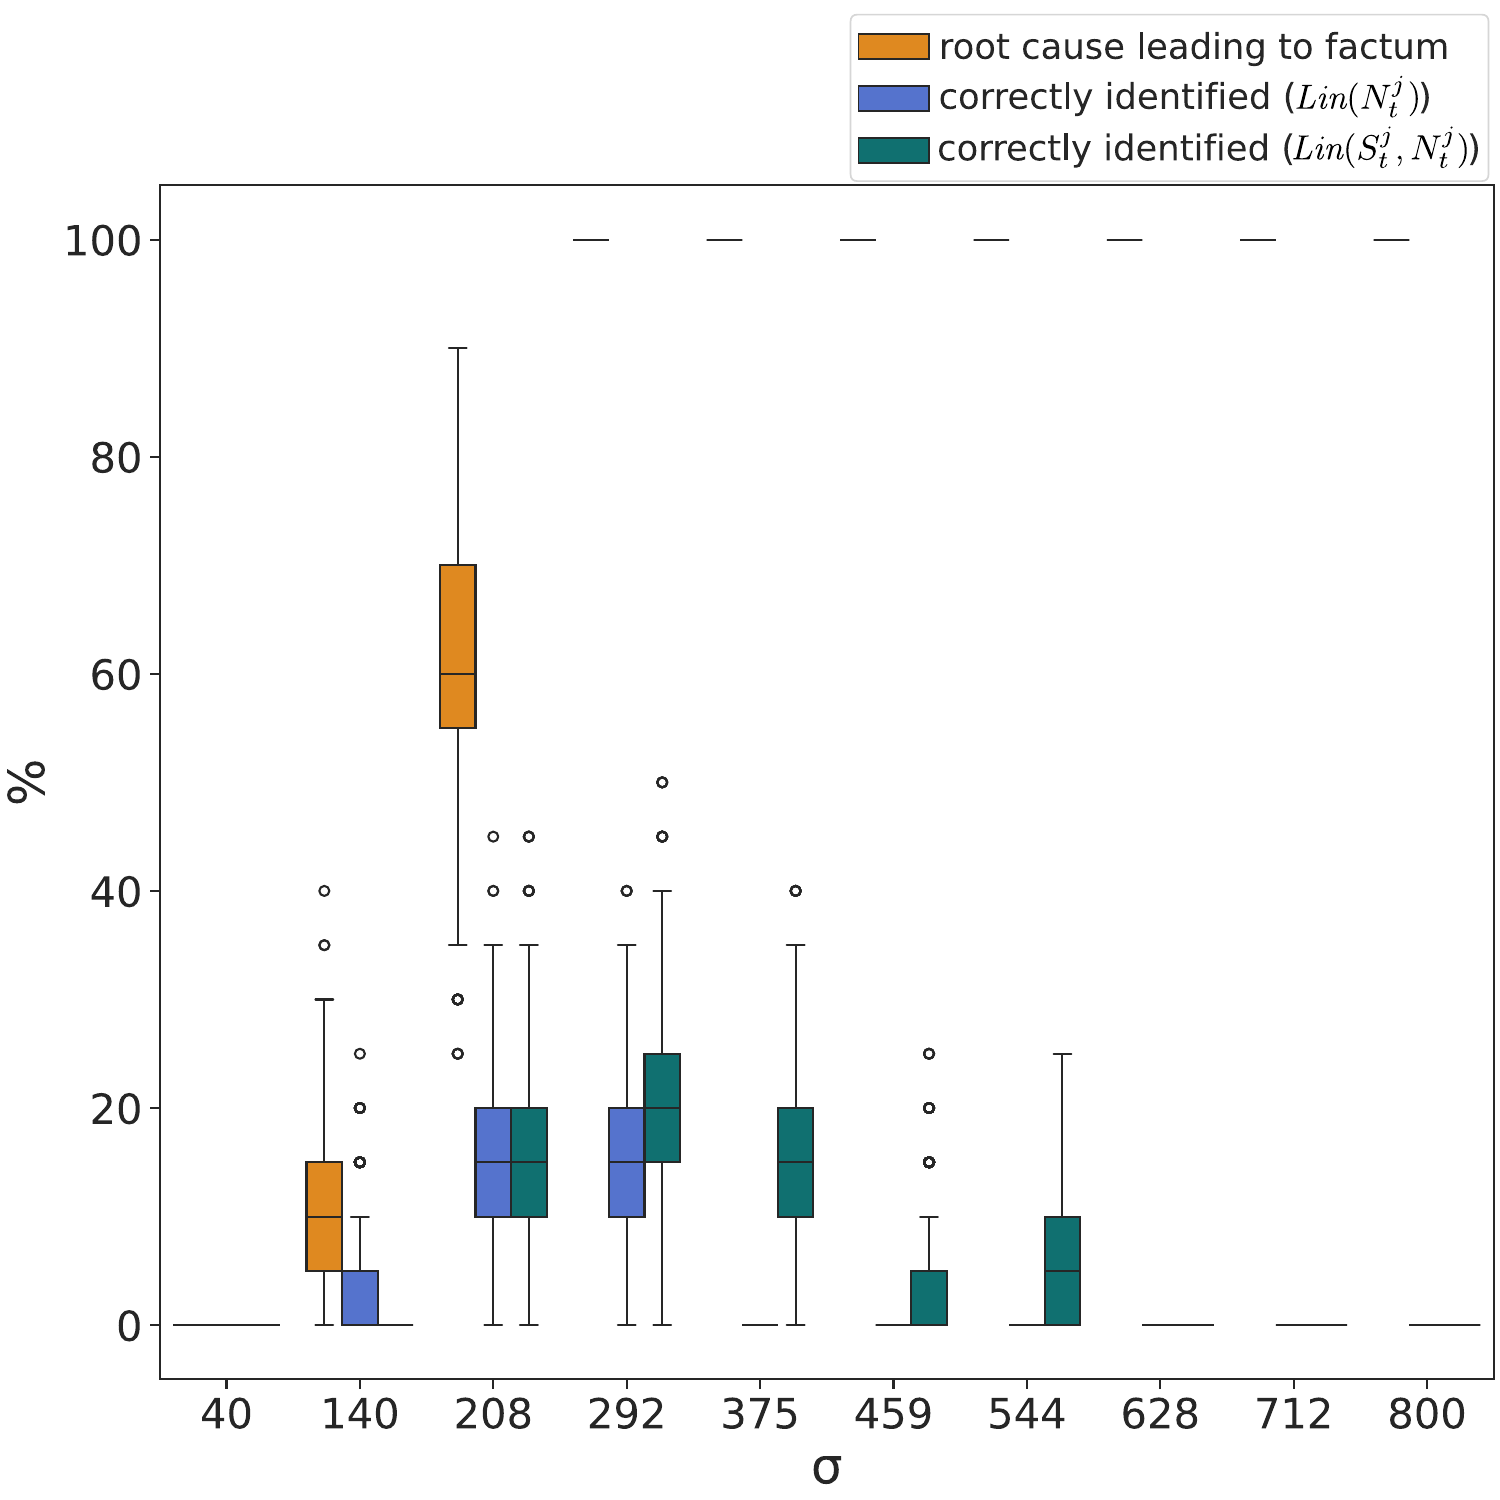}\label{fig:lin_model_oscillator_boxplot}}
    \caption{The root cause was injected at a random node $j=x_1$ at $t=24$ with varying constants in $[0.1,2.0]$. The x-axis shows the injected constant in relation to the noise standard deviation denoted by $\sigma$. We report how many root causes could be identified in \%.}
\label{fig:injection-boxplot-FHN}
\end{figure}

\end{document}
